# Supplementary material for: Pursuing Overall Welfare in Federated Learning through Sequential Decision Making
Source: arXiv:2405.20821 source file (2024-11-18)
Supplement: Supplementary file 1 [file e_convergence_analysis.tex]

\section{Convergence Analysis}
In this section, we present the convergence behavior of the whole FL system equipped with \texttt{AAggFF}.
\subsection{Notations}
Denote the FL objective (\ref{eq:fl_obj}) as $\min_{\boldsymbol{\theta}} {F}(\boldsymbol{\theta})\triangleq \sum_{i=1}^K p_i F_i(\boldsymbol{\theta})$, 
where $ F_i(\boldsymbol{\theta})=\mathbb{E}_{\xi\sim\mathcal{D}_i}[l(\xi;\boldsymbol{\theta})]$.

%Denote $\boldsymbol{\theta}^\star \triangleq \argmin_{\boldsymbol{\theta}\in\mathbb{R}^d} F(\boldsymbol{\theta})$.
Denote $\rho$ as the transformation defined as $\rho(x)=\texttt{CDF}(x)$ for an arbitrary cumulative distribution function (CDF), similar to (\ref{eq:resp_vec}).

Denote $\tilde{F}(\boldsymbol{\theta})\triangleq \sum_{i=1}^K p_i \tilde{F}_i(\boldsymbol{\theta})$,
where $\tilde{F}_i(\boldsymbol{\theta}) = \rho(F_i(\boldsymbol{\theta}))$.

Denote $F^{(t)}(\boldsymbol{\theta}) \triangleq \sum_{i=1}^K p^{(t)}_i F_i(\boldsymbol{\theta})$
and $\tilde{F}^{(t)}(\boldsymbol{\theta}) \triangleq \sum_{i=1}^K p^{(t)}_i \tilde{F}_i(\boldsymbol{\theta})$,
with slight abuse of notations.

\subsection{System Level Objective}
Let us first define the loss function for the FL system, which will later be used for defining a system-level objective.

\begin{definition} (System Loss) The loss function for the FL system, $\mathcal{L}:\mathbb{R}^d \times \Delta_{K-1}$  is defined as follows.
\label{def:system_loss}
\begin{equation}
\begin{gathered}
\label{eq:system_loss}
    \mathcal{L}(\boldsymbol{\theta}, \boldsymbol{p}) 
    \triangleq
    \log \left(1 + \sum_{i=1}^K p_i \tilde{F}_i (\boldsymbol{\theta}) \right)
    =
    \log \left(1 + \tilde{F} (\boldsymbol{\theta}) \right),
\end{gathered}
\end{equation}
\end{definition}
\vspace{2pt}

\begin{remark} (Same Minimizer) Since $\log(\cdot)$ and $\rho(\cdot)$ in (\ref{eq:system_loss}) are monotonically increasing functions, the location of the achieved minimum is also preserved. 
i.e., 
$\argmin_{\boldsymbol{\theta}\in\mathbb{R}^d} F(\boldsymbol{\theta}) 
= 
\argmin_{\boldsymbol{\theta}\in\mathbb{R}^d} \tilde{F}(\boldsymbol{\theta})$.
Note that this also holds for $\rho^{(t)}(\cdot)$ defined in (\ref{eq:resp_vec}), 
but we simply leave only the CDF function for the brevity of discussion.
\end{remark}
\vspace{2pt}

\begin{remark} (Retrieval of Objectives) When $\boldsymbol{\theta}^{(t)}$ is a fixed value given in a specific time $t$, 
we can retrieve the objective for determining a mixing coefficient $\boldsymbol{p}$:
$\max_{\boldsymbol{p}\in\Delta_{K-1}} \mathcal{L}(\boldsymbol{\theta}^{(t)}, \boldsymbol{p})
\equiv
\min_{\boldsymbol{p}\in\Delta_{K-1}} \ell^{(t)}(\boldsymbol{p})$,
where $\ell^{(t)}(\cdot)$ is a decision loss defined in (\ref{eq:decision_loss}), which is a negative of the system loss.
Similarly, when $\boldsymbol{p}^{(t)}$ is a fixed value given in a specific time $t$, 
we can retrieve the objective for optimizing a global parameter, $\boldsymbol{\theta}$:
$\min_{\boldsymbol{\theta}\in\mathbb{R}^K} \mathcal{L}(\boldsymbol{p}^{(t)}, \boldsymbol{\theta})
\equiv
\min_{\boldsymbol{\theta}\in\mathbb{R}^K} \tilde{F}^{(t)}(\boldsymbol{\theta})$.
\end{remark}
\vspace{4pt}

From now on, we denote the entire objective of FL system as a minimax formulation as follows.
\begin{equation}
\label{eq:system_objective}
    \min_{\boldsymbol{\theta}\in\mathbb{R}^d} \max_{\boldsymbol{p}\in\Delta_{K-1}} 
    \mathcal{L}(\boldsymbol{\theta}, \boldsymbol{p})
\end{equation}
It is a natural choice since in \texttt{AAggFF}, it first updates a mixing coefficient, 
and then updates a global model (i.e., central aggregation of local updates) using the updated mixing coefficient.
\vspace{4pt}

\begin{assumption} 
\label{assum:log_convexity}
(Log Convexity of Modified Global Objective) $\tilde{F}(\boldsymbol{\theta})$ is log-convex w.r.t. $\boldsymbol{\theta}\in\mathbb{R}^d$. i.e., $\log{(\tilde{F}(\boldsymbol{\theta}))}$ is convex w.r.t. $\boldsymbol{\theta}\in\mathbb{R}^d$.
\end{assumption}
\vspace{4pt}

\begin{assumption} (Diminishing Minimum Ratio) Assume for $\boldsymbol{\theta}'\in\mathbb{R}^d$, it holds that:
\begin{equation}
    \sum_{t=1}^T \frac{ 1 + {F}^{(t)}(\boldsymbol{\theta}') }{  1+ \tilde{F}^{(t)}(\boldsymbol{\theta}') } = o(T)
\end{equation}
\end{assumption}

Now, the system objective becomes a typical convex-concave minimax objective.
i.e., $\mathcal{L}$ is convex w.r.t. its first argument due to the Assumption~\ref{assum:log_convexity},
and concave w.r.t. its second argument which can be simply induced from the strict convexity of the decision loss (i.e., negative of the system loss), from Lemma~\ref{lemma:convexity}.
Then, a saddle point $(\boldsymbol{\theta}^*, \boldsymbol{p}^*)\in \mathbb{R}^d \times \Delta_{K-1}$ always exists \cite{existence}, which satisfies:
\begin{equation}
\begin{gathered}
    \mathcal{L}(\boldsymbol{\theta}^*, \boldsymbol{p})
    \triangleq
    \mathcal{L}(\boldsymbol{\theta}^*, \boldsymbol{p}^*)
    \leq
    \mathcal{L}(\boldsymbol{\theta}, \boldsymbol{p}^*),
    \quad \forall \boldsymbol{\theta} \in \mathbb{R}^d 
    \quad \text{ and } 
    \quad \forall \boldsymbol{p} \in \Delta_{K-1}.
\end{gathered}
\end{equation}
\vspace{4pt}

Next, let us define a criterion for checking a suboptimality of given solution $(\boldsymbol{\theta}', \boldsymbol{p}')\in\mathbb{R}^d \times \Delta_{K-1}$.
For the convex-concave minimax problem, a duality gap defined below is commonly used:
\begin{equation}
    \max_{\boldsymbol{p}\in\Delta_{K-1}} \mathcal{L}(\boldsymbol{\theta}', \boldsymbol{p}) 
    -
    \min_{\boldsymbol{\theta}\in\mathbb{R}^d} \mathcal{L}(\boldsymbol{\theta}, \boldsymbol{p}'),
    \quad \forall \boldsymbol{\theta}' \in \mathbb{R}^d 
    \quad \text{ and } 
    \quad \forall \boldsymbol{p}' \in \Delta_{K-1}.
\end{equation}

As a proxy for the duality gap in finite time $T$, we define and use the following system-level regret.
\begin{definition} (System-Level Regret) The system-level regret for \texttt{AAggFF} is defined over $(\boldsymbol{\theta}, \boldsymbol{p})\in\mathbb{R}^d \times \Delta_{K-1}$ in finite time $T$ as follows.
\begin{equation}
    \normalfont\text{Regret}^{(T)}\left(\boldsymbol{\theta}, \boldsymbol{p}\right)
    =
    \max_{\boldsymbol{p}\in\Delta_{K-1}} \sum_{t=1}^T \mathcal{L}(\boldsymbol{\theta}^{(t)}, \boldsymbol{p})
    -
    \min_{\boldsymbol{\theta}\in\mathbb{R}^K} \sum_{t=1}^T \mathcal{L}(\boldsymbol{\theta}, \boldsymbol{p}^{(t)}).
\end{equation}
Further define 
$\boldsymbol{\theta}_\star\triangleq\argmin_{\boldsymbol{\theta}\in\mathbb{R}^K} \sum_{t=1}^T \mathcal{L}(\boldsymbol{\theta}, \boldsymbol{p}^{(t)})$, and
$\boldsymbol{p}_\star\triangleq\argmax_{\boldsymbol{p}\in\Delta_{K-1}} \sum_{t=1}^T \mathcal{L}(\boldsymbol{\theta}^{(t)}, \boldsymbol{p})$.
\end{definition}

Then, we can also decompose the system-level regret as follows.
\begin{lemma} 
\label{lemma:decom_regret}
The system-level regret can be upper bounded as follows:
\begin{equation}
\begin{gathered}
    \normalfont\text{Regret}^{(T)}\left(\boldsymbol{\theta}_\star, \boldsymbol{p}_\star\right)
    =
    \sum_{t=1}^T \mathcal{L}(\boldsymbol{\theta}^{(t)}, \boldsymbol{p}_\star)
    -
    \sum_{t=1}^T \mathcal{L}(\boldsymbol{\theta}_\star, \boldsymbol{p}^{(t)}) \\
    \leq
    \left(
        \sum_{t=1}^T \ell^{(t)}(\boldsymbol{p}^{(t)})
        -
        \sum_{t=1}^T \ell^{(t)}(\boldsymbol{p}_\star)
    \right)
    +
    \left(
        \sum_{t=1}^T {F}^{(t)}(\boldsymbol{\theta}^{(t)})
        -
        \sum_{t=1}^T {F}^{(t)}(\boldsymbol{\theta}_\star)
    \right)
    +
    \left(
        \sum_{t=1}^T \frac{ 1 + {F}^{(t)}(\boldsymbol{\theta}_\star) }{  1+ \tilde{F}^{(t)}(\boldsymbol{\theta}_\star) }
    \right)
\end{gathered}
\end{equation}
\end{lemma}

\begin{proof}
In a round $t\in[T]$, we have:
\begin{equation}
\begin{split}
    \mathcal{L}(\boldsymbol{\theta}^{(t)}, \boldsymbol{p})
    -
    \mathcal{L}(\boldsymbol{\theta}, \boldsymbol{p}^{(t)}) \\
    &=
    \mathcal{L}(\boldsymbol{\theta}^{(t)}, \boldsymbol{p})
    -
    \mathcal{L}(\boldsymbol{\theta}^{(t)}, \boldsymbol{p}^{(t)})
    +
    \mathcal{L}(\boldsymbol{\theta}^{(t)}, \boldsymbol{p}^{(t)})
    -
    \mathcal{L}(\boldsymbol{\theta}, \boldsymbol{p}^{(t)}) \\
    &=
    \left(-\ell^{(t)}(\boldsymbol{p}) + \ell^{(t)}(\boldsymbol{p}^{(t)})\right)
    +
    \left(\mathcal{L}(\boldsymbol{\theta}^{(t)}, \boldsymbol{p}^{(t)})
    -
    \mathcal{L}(\boldsymbol{\theta}, \boldsymbol{p}^{(t)})\right) \\
    &=
    \left(\ell^{(t)}(\boldsymbol{p}^{(t)})-\ell^{(t)}(\boldsymbol{p})\right)
    +
    \log\left( \frac{ 1+\tilde{F}^{(t)}(\boldsymbol{\theta}^{(t)}) }{ 1+\tilde{F}^{(t)}(\boldsymbol{\theta}) } \right) \\
    &\leq
    \left(\ell^{(t)}(\boldsymbol{p}^{(t)})-\ell^{(t)}(\boldsymbol{p})\right)
    +
    \left( 
        \frac{ \tilde{F}^{(t)}(\boldsymbol{\theta}^{(t)}) - \tilde{F}^{(t)}(\boldsymbol{\theta}) }
        { 1+\tilde{F}^{(t)}(\boldsymbol{\theta}) } 
    \right) \\
    &\leq
    \left(\ell^{(t)}(\boldsymbol{p}^{(t)})-\ell^{(t)}(\boldsymbol{p})\right)
    +
    \left( 
        \frac{ 1 + {F}^{(t)}(\boldsymbol{\theta}^{(t)}) - \tilde{F}^{(t)}(\boldsymbol{\theta}) }
        { 1+\tilde{F}^{(t)}(\boldsymbol{\theta}) }
    \right) \\
    &=
    \left(\ell^{(t)}(\boldsymbol{p}^{(t)})-\ell^{(t)}(\boldsymbol{p})\right)
    +
    \frac{
        \left({F}^{(t)}(\boldsymbol{\theta}^{(t)}) - {F}^{(t)}(\boldsymbol{\theta}) \right)
        +
        \left( {F}^{(t)}(\boldsymbol{\theta}) - \tilde{F}^{(t)}(\boldsymbol{\theta}) \right)
        +
        1
    }
    { 1+\tilde{F}^{(t)}(\boldsymbol{\theta}) } \\
    &\leq
    \left(\ell^{(t)}(\boldsymbol{p}^{(t)})-\ell^{(t)}(\boldsymbol{p})\right)
    +
    \left({F}^{(t)}(\boldsymbol{\theta}^{(t)}) - {F}^{(t)}(\boldsymbol{\theta}) \right)
    +    
    \frac{ 1 + {F}^{(t)}(\boldsymbol{\theta}) }{  1+ \tilde{F}^{(t)}(\boldsymbol{\theta}) },
\end{split}
\end{equation}
where the first inequality is due to the inequality $\log(x)\leq x-1$,
the second inequality is from the fact that any \texttt{CDF} can be upper bounded by $x+1$, i.e., $\rho(x)\leq x+1,  \forall x\geq0$,
and the third inequality is trivial since $\tilde{F}^{(t)}(\boldsymbol{\theta})$ is non-negative.
Now summing up for $t\in[T]$, we have
\begin{equation}
\begin{gathered}
    \sum_{t=1}^T \mathcal{L}(\boldsymbol{\theta}^{(t)}, \boldsymbol{p})
    -
    \sum_{t=1}^T \mathcal{L}(\boldsymbol{\theta}, \boldsymbol{p}^{(t)}) \\
    \leq
    \left(
        \sum_{t=1}^T \ell^{(t)}(\boldsymbol{p}^{(t)})
        -
        \sum_{t=1}^T \ell^{(t)}(\boldsymbol{p})
    \right)
    +
    \left(
        \sum_{t=1}^T {F}^{(t)}(\boldsymbol{\theta}^{(t)})
        -
        \sum_{t=1}^T {F}^{(t)}(\boldsymbol{\theta})
    \right)
    +
    \left(
        \sum_{t=1}^T \frac{ 1 + {F}^{(t)}(\boldsymbol{\theta}) }{  1+ \tilde{F}^{(t)}(\boldsymbol{\theta}) }
    \right)
\end{gathered}
\end{equation}
Finally, plugging $(\boldsymbol{\theta}_\star, \boldsymbol{p}_\star)$ into $(\boldsymbol{\theta}, \boldsymbol{p})$,
we have the statement.
\end{proof}

\begin{remark} (Decomposed Regret Upper Bound) Let us inspect decomposed system-level regret upper bound in Lemma~\ref{lemma:decom_regret}.
The first term is a familiar term and we already know the upper bound, viz. the regret upper bound in Theorem~\ref{thm:crosssilo} and Theorem~\ref{thm:crossdevice_full}).
Let us defer discussion of the second term to the Section~\ref{subsec:theta}.
The third term is 
\end{remark}

\subsection{Convergence Bound for $\boldsymbol{\theta}$}
\label{subsec:theta}
\begin{assumption} 
\label{assum:unbaised_grad}
(Unbiased Local Gradient) The stochastic gradient calculated at each client, 
denoted as $\nabla l(\xi;\boldsymbol{\theta})$, where $\xi$ is a local data sampled from local dataset $\mathcal{D}_i$, is an unbiased estimator of the gradient of local objective. 
i.e., $\mathbb{E}_{\xi\sim\mathcal{D}_i} [\nabla l(\xi;\boldsymbol{\theta})] = \nabla F_i(\boldsymbol{\theta}), \forall i \in [K]$.   
\end{assumption}

\begin{assumption} 
\label{assum:lipschitz}
(Lipschitz Local Objective) For any $i, j\in[K]$, $F_i - F_j$ is $\sigma$-Lipschitz continuous w.r.t. $\Vert\cdot\Vert_2$.
\end{assumption}

\begin{assumption} 
\label{assum:bounded_var}
(Bounded Variance) The stochastic gradient calculated at each client has a bounded variance, $\sigma^2 \geq 0$.
i.e., $\mathbb{E}_{\xi\sim\mathcal{D}_i} [\Vert \nabla l(\xi;\boldsymbol{\theta}) - \nabla F_i(\boldsymbol{\theta}) \Vert^2] \leq \sigma_i^2, \forall \boldsymbol{\theta} \in \mathbb{R}^d$.
\end{assumption}

\begin{assumption}
\label{assum:smooth}
($G$-smooth Function bounded Below) Each local objective $F_i$ is $G$-smooth. For all $\boldsymbol{\theta}, \boldsymbol{\theta}' \in \mathbb{R}^d$, the local objective satisfies 
$\Vert \nabla F_i(\boldsymbol{\theta}) - \nabla F_i(\boldsymbol{\theta}') \Vert \leq G \Vert \boldsymbol{\theta} - \boldsymbol{\theta}' \Vert^2, \forall i \in [K]$.
Further assume that $F(\cdot)$ is bounded below by the function $F_*$.
\end{assumption}

\begin{assumption} 
\label{assum:pl}
($M$-PL condition \cite{pl}) The global objective $F$ satisfies the Polyak-Łojasiewicz (PL) condition for some $M > 0$. 
In other words, it satisfies $\Vert \nabla F(\boldsymbol{\theta}) \Vert^2 \geq 2M \left(F(\boldsymbol{\theta}) - F(\boldsymbol{\theta}_\star)\right), 
\forall \boldsymbol{\theta} \in \mathbb{R}^d$.
\end{assumption}

\begin{lemma}
\begin{equation}
    \sum_{t=1}^T {F}^{(t)}(\boldsymbol{\theta}^{(t)})
    -
    \sum_{t=1}^T {F}^{(t)}(\boldsymbol{\theta}_\star)
    \leq
    \mathcal{O}(T)?
\end{equation}
\end{lemma}

\begin{proof}
While we assume full-client participation setting for the ease of discussion, it can be easily extended to the partial client participation setting, e.g., see the proof of Theorem 4.2 of \cite{propfair}.
Denote $\boldsymbol{\theta}^{(t)}_{i,j-1}$ as the model parameter of $i$-th client in round $t$ at $j$-th local update,
where we set $\boldsymbol{\theta}^{(t)}_{i,0}\leftarrow\boldsymbol{\theta}^{(t)}$.
Denote further that a stochastic gradient calculated at each client $i\in[K]$ in $t\in[T]$ as $\boldsymbol{d}^{(t)}_{i,j} \triangleq \nabla l(\Xi_{i,j},\boldsymbol{\theta}^{(t)}_{i,j-1})$, 
where $\Xi_{i,j}$ is a $j$-th ($j\in[J]$) local mini-batch of size $B$, independently and identically sampled from local dataset $\mathcal{D}_i$. (i.e., $J$ is number of local updates)

Then, we can write the model aggregation step at the central server as follows.
\begin{equation}
\begin{gathered}
    \boldsymbol{\theta}^{(t+1)}=\sum_{i=1}^K p^{(t+1)}_i \boldsymbol{\theta}^{(t)}_{i,J}.
\end{gathered}
\end{equation}
Accordingly, the local update can be written as:
\begin{equation}
\begin{gathered}
    \boldsymbol{\theta}^{(t)}_{i,j}=\boldsymbol{\theta}^{(t)}_{i,j-1}-\eta\boldsymbol{d}^{(t)}_{i,j}, \quad \forall j\in[J],
\end{gathered}
\end{equation}
where $\eta$ is a local learning rate.

Thus, we can re-write the model aggregation step as follows.
\begin{equation}
\begin{gathered}
\label{eq:server_agg_formula}
    \boldsymbol{\theta}^{(t+1)}=\boldsymbol{\theta}^{(t)}-\eta\sum_{i=1}^K p_i^{(t+1)} \sum_{j=1}^J \boldsymbol{d}^{(t)}_{i,j}.
\end{gathered}
\end{equation}

From the Assumption~\ref{assum:smooth}, the global objective $F$ is also said to be $G$-smooth.
Thus, we have:
\begin{equation}
\begin{gathered}
    F(\boldsymbol{\theta}^{(t+1)}) 
    \leq 
    F(\boldsymbol{\theta}^{(t)})
    +
    \left\langle\nabla F(\boldsymbol{\theta}^{(t)}), \boldsymbol{\theta}^{(t+1)} - \boldsymbol{\theta}^{(t)} \right\rangle
    +
    \frac{G}{2}\left\Vert \boldsymbol{\theta}^{(t+1)} - \boldsymbol{\theta}^{(t)} \right\Vert^2.
\end{gathered}
\end{equation}

Combined with (\ref{eq:server_agg_formula}), it becomes:
{\allowdisplaybreaks
\begin{align*}
    &F(\boldsymbol{\theta}^{(t+1)}) 
    \leq 
    F(\boldsymbol{\theta}^{(t)})
    -\eta
    \left\langle\nabla F(\boldsymbol{\theta}^{(t)}), \sum_{i=1}^K p_i^{(t+1)} \sum_{j=1}^J \boldsymbol{d}^{(t)}_{i,j} \right\rangle
    +
    \frac{\eta^2 G}{2}\left\Vert \sum_{i=1}^K p_i^{(t+1)} \sum_{j=1}^J \boldsymbol{d}^{(t)}_{i,j} \right\Vert^2 \\
    &=
    F(\boldsymbol{\theta}^{(t)})
    -\eta
    \left\langle\nabla F(\boldsymbol{\theta}^{(t)}), 
    \sum_{i=1}^K p_i^{(t+1)} \sum_{j=1}^J \left(\boldsymbol{d}^{(t)}_{i,j}-\nabla F(\boldsymbol{\theta}^{(t)}) + \nabla F(\boldsymbol{\theta}^{(t)})\right) \right\rangle \\
    &+
    \frac{\eta^2 G}{2}
    \left\Vert \sum_{i=1}^K p_i^{(t+1)} \sum_{j=1}^J \left(\boldsymbol{d}^{(t)}_{i,j}-\nabla F(\boldsymbol{\theta}^{(t)}) + \nabla F(\boldsymbol{\theta}^{(t)})\right) \right\Vert^2 \\
    =
    &F(\boldsymbol{\theta}^{(t)})
    -\eta J \Vert \nabla F(\boldsymbol{\theta}^{(t)}) \Vert^2
    -\eta \left\langle\nabla F(\boldsymbol{\theta}^{(t)}), 
    \sum_{i=1}^K p_i^{(t+1)} \sum_{j=1}^J \left(\boldsymbol{d}^{(t)}_{i,j}-\nabla F(\boldsymbol{\theta}^{(t)})\right) \right\rangle \\
    &+
    \frac{\eta^2 G}{2}
    \left\Vert \sum_{i=1}^K p_i^{(t+1)} \sum_{j=1}^J \left(\boldsymbol{d}^{(t)}_{i,j}-\nabla F(\boldsymbol{\theta}^{(t)})\right) + J \nabla F(\boldsymbol{\theta}^{(t)}) \right\Vert^2 \\
    =
    &F(\boldsymbol{\theta}^{(t)})
    -\eta J \Vert \nabla F(\boldsymbol{\theta}^{(t)}) \Vert^2
    -\eta \left\langle\nabla F(\boldsymbol{\theta}^{(t)}), 
    \sum_{i=1}^K p_i^{(t+1)} \sum_{j=1}^J \left(\boldsymbol{d}^{(t)}_{i,j}-\nabla F(\boldsymbol{\theta}^{(t)})\right) \right\rangle \\
    &+
    \frac{\eta^2 G}{2}
    \left\Vert \sum_{i=1}^K p_i^{(t+1)} \sum_{j=1}^J \left( \boldsymbol{d}^{(t)}_{i,j} -\nabla F(\boldsymbol{\theta}^{(t)}) \right) \right\Vert^2 \\
    &+\eta^2 G J
    \left\langle 
        \sum_{i=1}^K p_i^{(t+1)} \sum_{j=1}^J \left(\boldsymbol{d}^{(t)}_{i,j}-\nabla F(\boldsymbol{\theta}^{(t)})\right),
        \nabla F(\boldsymbol{\theta}^{(t)}) 
    \right\rangle
    +\frac{\eta^2 G J^2}{2} 
    \Vert \nabla F(\boldsymbol{\theta}^{(t)}) \Vert^2
\end{align*}
}
Grouping similar terms together, we have:
\begin{equation}
\begin{gathered}
    F(\boldsymbol{\theta}^{(t+1)}) 
    \leq 
    F(\boldsymbol{\theta}^{(t)})
    -\eta J \left(1-\frac{\eta G J}{2}\right) \Vert \nabla F(\boldsymbol{\theta}^{(t)}) \Vert^2 \\
    -\eta ( 1 - \eta G J) \left\langle\nabla F(\boldsymbol{\theta}^{(t)}), 
    \sum_{i=1}^K p_i^{(t+1)} \sum_{j=1}^J \left(\boldsymbol{d}^{(t)}_{i,j}-\nabla F(\boldsymbol{\theta}^{(t)})\right) \right\rangle
    +
    \frac{\eta^2 G}{2}
    \left\Vert \sum_{i=1}^K p_i^{(t+1)} \sum_{j=1}^J \left( \boldsymbol{d}^{(t)}_{i,j} -\nabla F(\boldsymbol{\theta}^{(t)}) \right) \right\Vert^2. 
\end{gathered}
\end{equation}
Taking expectation on both sides, and sequentially applying the Cauchy-Schwarz inequality, and AM-GM inequality on the inner product term, we have:
\begin{equation}
\begin{gathered}
    \mathbb{E} [F(\boldsymbol{\theta}^{(t+1)})] 
    \leq 
    \mathbb{E} [F(\boldsymbol{\theta}^{(t)})]
    -\eta J \left(1-\frac{\eta G J}{2}\right) \mathbb{E}[\Vert \nabla F(\boldsymbol{\theta}^{(t)}) \Vert^2] \\
    +\eta ( 1 - \eta G J) \mathbb{E} \left[
        \Vert \nabla F(\boldsymbol{\theta}^{(t)}) \Vert \cdot
        \left\Vert \sum_{i=1}^K p_i^{(t+1)} \sum_{j=1}^J \left(\nabla F_i(\boldsymbol{\theta}^{(t)}_{i,j-1})-\nabla F(\boldsymbol{\theta}^{(t)})\right) \right\Vert
    \right] \\
    +
    \frac{\eta^2 G}{2}
    \mathbb{E}\left[
        \left\Vert \sum_{i=1}^K p_i^{(t+1)} \sum_{j=1}^J \left( \boldsymbol{d}^{(t)}_{i,j} -\nabla F(\boldsymbol{\theta}^{(t)}) \right) \right\Vert^2
    \right]. 
\end{gathered}
\end{equation}
By the AM-GM inequality, we have:
\begin{equation}
\begin{gathered}
    \mathbb{E} [F(\boldsymbol{\theta}^{(t+1)})] 
    \leq 
    \mathbb{E} [F(\boldsymbol{\theta}^{(t)})]
    -
    \left( \eta J \left(1-\frac{\eta G J}{2}\right) - \frac{\eta ( 1 - \eta G J)}{2 }\right) 
    \mathbb{E}[\Vert \nabla F(\boldsymbol{\theta}^{(t)}) \Vert^2] \\
    +\frac{\eta ( 1 - \eta G J)}{2} 
        \underbrace{ \mathbb{E} \left[
            \left\Vert \sum_{i=1}^K p_i^{(t+1)} \sum_{j=1}^J \left(\nabla F_i(\boldsymbol{\theta}^{(t)}_{i,j-1})-\nabla F(\boldsymbol{\theta}^{(t)})\right) \right\Vert^2
        \right]
    }_{(i)} \\
    +
    \frac{\eta^2 G}{2}
    \underbrace{
        \mathbb{E}\left[
            \left\Vert \sum_{i=1}^K p_i^{(t+1)} \sum_{j=1}^J \left( \boldsymbol{d}^{(t)}_{i,j} -\nabla F(\boldsymbol{\theta}^{(t)}) \right) \right\Vert^2
        \right]
    }_{(ii)}. 
\end{gathered}
\end{equation}

By directly applying the result of ((B.23) of \cite{propfair}), we can bound (i) as:
\begin{equation}
\begin{gathered}
\label{eq:in_mid_of_second_term}
    \mathbb{E} \left[
        \left\Vert \sum_{i=1}^K p_i^{(t+1)} \sum_{j=1}^J \left(\nabla F_i(\boldsymbol{\theta}^{(t)}_{i,j-1})-\nabla F(\boldsymbol{\theta}^{(t)})\right) \right\Vert^2
    \right] \\
    \leq
    K J^2 \sigma^2 \Vert \boldsymbol{p}^{(t+1)} \Vert^2_2 
    + 2 K G^2 J \Vert \boldsymbol{p}^{(t+1)} \Vert^2_2 \sum_{i=1}^K \sum_{j=1}^J \mathbb{E}[\Vert\boldsymbol{\theta}^{(t)}_{i,j-1} - \boldsymbol{\theta}^{(t)}\Vert^2] \\
    \leq
    K J^2 \sigma^2
    + 2 K G^2 J \sum_{i=1}^K \sum_{j=1}^J \mathbb{E}[\Vert\boldsymbol{\theta}^{(t)}_{i,j-1} - \boldsymbol{\theta}^{(t)}\Vert^2],
\end{gathered}
\end{equation}
using the following identity $\nabla F_i(\boldsymbol{\theta}^{(t)}_{i,j-1})-\nabla F(\boldsymbol{\theta}^{(t)})
= \nabla F_i(\boldsymbol{\theta}^{(t)}_{i,j-1}) -\nabla F_i(\boldsymbol{\theta}^{(t)}) + \nabla F_i(\boldsymbol{\theta}^{(t)}) -\nabla F(\boldsymbol{\theta}^{(t)})$ in the first inequality,
and the second inequality is due to $\Vert \boldsymbol{p} \Vert_2 \leq \Vert \boldsymbol{p} \Vert_1 =1, \forall \boldsymbol{p}\in\Delta_{K-1}$.

Again applying the previous results of ((B.16) of \cite{propfair}), we can bound (ii) as:
\begin{equation}
\begin{gathered}
    \mathbb{E}\left[
        \left\Vert \sum_{i=1}^K p_i^{(t+1)} \sum_{j=1}^J \left( \boldsymbol{d}^{(t)}_{i,j} -\nabla F(\boldsymbol{\theta}^{(t)}) \right) \right\Vert^2
    \right]
    \leq
    \frac{K J}{B} \Vert \boldsymbol{p}^{(t+1)} \Vert^2_2 \sum_{i=1}^K \sigma_i^2
    \leq
    \frac{K J}{B} \sum_{i=1}^K \sigma_i^2,
\end{gathered}
\end{equation}
using the following identity 
$\boldsymbol{d}^{(t)}_{i,j} -\nabla F(\boldsymbol{\theta}^{(t)})
=\boldsymbol{d}^{(t)}_{i,j} - \nabla F_i(\boldsymbol{\theta}^{(t)}_{i,j-1}) + \nabla F_i(\boldsymbol{\theta}^{(t)}_{i,j-1}) -\nabla F(\boldsymbol{\theta}^{(t)})$ in the first inequality,
and the second inequality is due to $\Vert \boldsymbol{p} \Vert_2 \leq \Vert \boldsymbol{p} \Vert_1 =1, \forall \boldsymbol{p}\in\Delta_{K-1}$.

For bounding the last term in (\ref{eq:in_mid_of_second_term}), we use the previous result, (B.29) of \cite{propfair}.
\begin{equation}
\begin{gathered}
    \mathbb{E}[\Vert\boldsymbol{\theta}^{(t)}_{i,j} - \boldsymbol{\theta}^{(t)}\Vert^2]
    \leq
    \left( 1 + \frac{1}{2J-1} + 6G^2J\eta^2 \right)
    \mathbb{E}[\Vert\boldsymbol{\theta}^{(t)}_{i,j-1} - \boldsymbol{\theta}^{(t)}\Vert^2]
    +
    \left( 6\sigma^2 J + \frac{\sigma_i^2}{B} \right)
    +
    6J\eta^2 \mathbb{E}[\Vert\nabla F(\boldsymbol{\theta}^{(t)})\Vert^2].
\end{gathered}
\end{equation}
Assuming that $\eta\leq\frac{1}{6GJ}$, we can further use the result of (B.33) of \cite{propfair}.
\begin{equation}
\begin{gathered}
    \sum_{j=0}^{J-1} \mathbb{E}[\Vert\boldsymbol{\theta}^{(t)}_{i,j} - \boldsymbol{\theta}^{(t)}\Vert^2]
    \leq
    (e - 2)J^2\eta^2\left( 6 \sigma^2 J + \frac{\sigma_i^2}{B} + 6 J \mathbb{E}[\Vert\nabla F(\boldsymbol{\theta}^{(t)})\Vert^2]  \right).
\end{gathered}
\end{equation}

Combining all, we have following upper bound:
{\allowdisplaybreaks
\begin{align*}
    &\mathbb{E} [F(\boldsymbol{\theta}^{(t+1)})] 
    \leq 
    \mathbb{E} [F(\boldsymbol{\theta}^{(t)})]
    -
    \left( \eta J \left(1-\frac{\eta G J}{2}\right) - \frac{\eta ( 1 - \eta G J)}{2 }\right) 
    \mathbb{E}[\Vert \nabla F(\boldsymbol{\theta}^{(t)}) \Vert^2] \\
    &+\frac{\eta ( 1 - \eta G J)}{2} 
    \mathbb{E} \left[
        \left\Vert \sum_{i=1}^K p_i^{(t+1)} \sum_{j=1}^J \left(\nabla F_i(\boldsymbol{\theta}^{(t)}_{i,j-1})-\nabla F(\boldsymbol{\theta}^{(t)})\right) \right\Vert^2
    \right] \\
    &+
    \frac{\eta^2 G}{2}
    \mathbb{E}\left[
        \left\Vert \sum_{i=1}^K p_i^{(t+1)} \sum_{j=1}^J \left( \boldsymbol{d}^{(t)}_{i,j} -\nabla F(\boldsymbol{\theta}^{(t)}) \right) \right\Vert^2
    \right] \\
    &=
    \mathbb{E} [F(\boldsymbol{\theta}^{(t)})]
    -
    \left( \eta J \left(1-\frac{\eta G J}{2}\right) - \frac{\eta ( 1 - \eta G J)}{2 }\right) 
    \mathbb{E}[\Vert \nabla F(\boldsymbol{\theta}^{(t)}) \Vert^2] \\
    &+\left(\frac{\eta^2 G}{2} + \frac{\eta ( 1 - \eta G J)}{2}\right) 
    \mathbb{E} \left[
        \left\Vert \sum_{i=1}^K p_i^{(t+1)} \sum_{j=1}^J \left(\nabla F_i(\boldsymbol{\theta}^{(t)}_{i,j-1})-\nabla F(\boldsymbol{\theta}^{(t)})\right) \right\Vert^2
    \right] \\
    &+
    \frac{\eta^2 G}{2}
    \mathbb{E}\left[
        \left\Vert \sum_{i=1}^K p_i^{(t+1)} \sum_{j=1}^J \left( \boldsymbol{d}^{(t)}_{i,j} -\nabla F_i(\boldsymbol{\theta}^{(t)}_{i,j-1}) \right) \right\Vert^2
    \right] \\
    &\leq
    \mathbb{E} [F(\boldsymbol{\theta}^{(t)})]
    -
    \left( \eta J \left(1-\frac{\eta G J}{2}\right) - \frac{\eta ( 1 - \eta G J)}{2 }\right) 
    \mathbb{E}[\Vert \nabla F(\boldsymbol{\theta}^{(t)}) \Vert^2] \\
    &+\frac{\eta ( 1 - \eta G J)}{2} 
    \mathbb{E} \left[
        \left\Vert \sum_{i=1}^K p_i^{(t+1)} \sum_{j=1}^J \left(\nabla F_i(\boldsymbol{\theta}^{(t)}_{i,j-1})-\nabla F(\boldsymbol{\theta}^{(t)})\right) \right\Vert^2
    \right] \\
    &+
    \frac{\eta^2 GKJ}{2B}
    \sum_{i=1}^K \sigma_i^2 \\
    &\leq
    \mathbb{E} [F(\boldsymbol{\theta}^{(t)})]
    -
    \left( \eta J \left(1-\frac{\eta G J}{2}\right) - \frac{\eta ( 1 - \eta G J)}{2 }\right) 
    \mathbb{E}[\Vert \nabla F(\boldsymbol{\theta}^{(t)}) \Vert^2] \\
    &+\frac{\eta}{2} 
    \mathbb{E} \left[
        \left\Vert \sum_{i=1}^K p_i^{(t+1)} \sum_{j=1}^J \left(\nabla F_i(\boldsymbol{\theta}^{(t)}_{i,j-1})-\nabla F(\boldsymbol{\theta}^{(t)})\right) \right\Vert^2
    \right] \\
    &+
    \frac{\eta^2 GKJ}{2B}
    \sum_{i=1}^K \sigma_i^2 \\
    &\leq
    \mathbb{E} [F(\boldsymbol{\theta}^{(t)})]
    -
    \left( \eta J \left(1-\frac{\eta G J}{2}\right) - \frac{\eta ( 1 - \eta G J)}{2 }\right) 
    \mathbb{E}[\Vert \nabla F(\boldsymbol{\theta}^{(t)}) \Vert^2] \\
    &+\frac{\eta}{2} 
    \left(
    K J^2 \sigma^2 + 12(e-2)K^2G^2J^4\sigma^2\eta^2 
    \right)
    +
    \frac{2(e-2)KG^2J^3\eta^2}{B} \sum_{i=1}^K \sigma_i^2 \\
    &
    +
    6(e-2)KG^2J^4\eta^3 \mathbb{E}[\Vert \nabla F(\boldsymbol{\theta}^{(t)}) \Vert^2]
    +
    \frac{\eta^2 GKJ}{2B}
    \sum_{i=1}^K \sigma_i^2 \\
    &\leq
    \mathbb{E} [F(\boldsymbol{\theta}^{(t)})]
    -
    \frac{11J-6}{12} \eta 
    \mathbb{E}[\Vert \nabla F(\boldsymbol{\theta}^{(t)}) \Vert^2] \\
    &+\frac{\eta}{2} 
    \left(
    K J^2 \sigma^2 + 12(e-2)K^2G^2J^4\sigma^2\eta^2 
    \right)
    +
    \frac{2(e-2)KG^2J^3\eta^2}{B} \sum_{i=1}^K \sigma_i^2 \\
    &
    +
    6(e-2)KG^2J^4\eta^3 \mathbb{E}[\Vert \nabla F(\boldsymbol{\theta}^{(t)}) \Vert^2]
    +
    \frac{\eta^2 GKJ}{2B}
    \sum_{i=1}^K \sigma_i^2 \\
    &\leq
    \mathbb{E} [F(\boldsymbol{\theta}^{(t)})]
    -
    \left( \frac{11J-6}{ 12} - 6(e-2)KG^2J^4\eta^2 \right)\eta \mathbb{E}[\Vert \nabla F(\boldsymbol{\theta}^{(t)}) \Vert^2] \\
    &+ 
    \frac{KJ\eta}{2}
    \left(
    J\sigma^2(1+12(e-2)KG^2J^2\eta^2) 
    +
    \frac{G}{B}\left(1+2(e-2)GJ^2\right)
    \sum_{i=1}^K \sigma_i^2\right)
\end{align*}
}

Denote $\Gamma = \frac{KJ\eta}{2} \left( J\sigma^2(1+12(e-2)KG^2J^2\eta^2) + \frac{G}{B}\left(1+2(e-2)GJ^2\right) \sum_{i=1}^K \sigma_i^2\right)$.
    
Further denote $\tilde{\eta} = \left( \frac{11J-6}{12} - 6(e-2)KG^2J^4\eta^2 \right)\eta$.

Suppose we set $\eta \leq \min\left\{ \frac{1}{6GJ}, \sqrt{\frac{11J-6}{72(e-2)KG^2J^4}} \right\}$, then by the Assumption~\ref{assum:pl}, we have:
\begin{equation}
\begin{gathered}
    \mathbb{E} [F(\boldsymbol{\theta}^{(t+1)})] 
    \leq 
    \mathbb{E} [F(\boldsymbol{\theta}^{(t)})]
    -
    2 M \tilde{\eta}  
    \left( \mathbb{E}[F(\boldsymbol{\theta}^{(t)})] - F(\boldsymbol{\theta}_\star) \right) + \Gamma.
\end{gathered}
\end{equation}
By subtracting $F(\boldsymbol{\theta}_\star)$ from both sides, we have:
\begin{equation}
\begin{gathered}
    \mathbb{E} [F(\boldsymbol{\theta}^{(t+1)})] - F(\boldsymbol{\theta}_\star)
    \leq 
    (1 - 2 M \tilde{\eta})  
    \left( \mathbb{E}[F(\boldsymbol{\theta}^{(t)})] - F(\boldsymbol{\theta}_\star) \right) + \Gamma.
\end{gathered}
\end{equation}
Recursively applying above with $M\leq\frac{1}{\tilde{\eta}}$, we have:
\begin{equation}
\begin{gathered}
    \mathbb{E} [F(\boldsymbol{\theta}^{(T)})] - F(\boldsymbol{\theta}_\star)
    \leq 
    (1 - 2 M \tilde{\eta})^T 
    \left( \mathbb{E}[F(\boldsymbol{\theta}^{(0)})] - F(\boldsymbol{\theta}_\star) \right) + \frac{1-{(1-2M\tilde{\eta})}^{T-1}}{2M\tilde{\eta}}\Gamma.
\end{gathered}
\end{equation}
\end{proof}
